# Supplementary material for: Multitaper Spectral Estimation HDP-HMMs for EEG Sleep Inference
Source: arXiv:1805.07300 ancillary file (2018-05-18)
Supplement: Supplementary file 1 [file MSEHDPHMM-Supplementary.pdf]

# Multitaper Spectral Estimation HDP-HMMs for EEG Sleep Inference
# (Supplementary Material)

**Leon Chlon***
MIT Department of BCS
Cambridge, MA 02139
lchlon@mit.edu

**Andrew H. Song***
MIT Department of EECS
Cambridge, MA 02139
andrew90@mit.edu

**Sandya Subramanian**
Harvard-MIT HST
Cambridge, MA 02139
sandya@mit.edu

**Hugo Soulat**
MIT Department of BCS
Cambridge, MA 02139
hsoulat@mit.edu

**John Tauber**
MIT Department of BCS
Cambridge, MA 02139
jtauber@mit.edu

**Demba Ba**
SEAS Department of Harvard
Cambridge, MA 02138
demba@seas.harvard.edu

**Michael Prerau**
MGH Department of Anesthesia, Critical Care and Pain Medicine
55 Fruit st, GRJ 4, Boston, MA 02114
prerau@nmr.mgh.harvard.edu

## 1 Additional Details: Proposition 1

Power Spectral Density (PSD), $f(w_j)$, denotes the power distribution of a WSS stochastic process over frequency. By virtue of the celebrated Wiener-Khinchin theorem [1], the expected value of power at $w_j$ of a realized time series converges to $f(w_j)$ as $J \to \infty$.

This lemma justifies the asymptotic independence of DFT coefficients across different frequencies, as well as between the real and imaginary parts within the same frequency. In this study, $J = 3,000$ (15 seconds/window with 200 Hz sampling rate) gives us a reasonable confidence in using the asymptotic normality &independence.

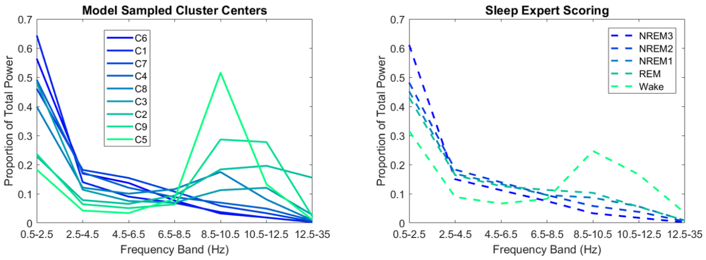


Figure S1: Model Sampled Cluster Centers vs Sleep Expert Scored Stages. Left: PSD of the centers of each of the seven discovered clusters, by proportion of total power in each frequency band. Right: PSD of each of the sleep expert scored stages, by averaging all windows (across subjects) scored as each state in terms of proportion of total power in each frequency band.

*These authors contributed equally to this work.

Preprint. Work in progress.

# 2 Additional Details: Simulated data

$D = 5$ sleep-inspired stages are generated. We model a slow oscillation ($f_{so} = 0.2$Hz), delta ($f_\delta = 3$ Hz), theta ($f_\theta = 5$Hz), alpha ($f_\alpha = 10$Hz) and sigma ($f_\sigma = 14$Hz). The periodograms and both multitapered and theoretical PSD for each stage are illustrated on the left plots of Figure S2. We report the HDP-HMM error estimate of discrete spectral characteristics (between the fitted discrete spectral contents and the median power for each frequency bands in dB) for both the periodogram and multitaper methods for each state and frequency band in the right plots of Figure S2.

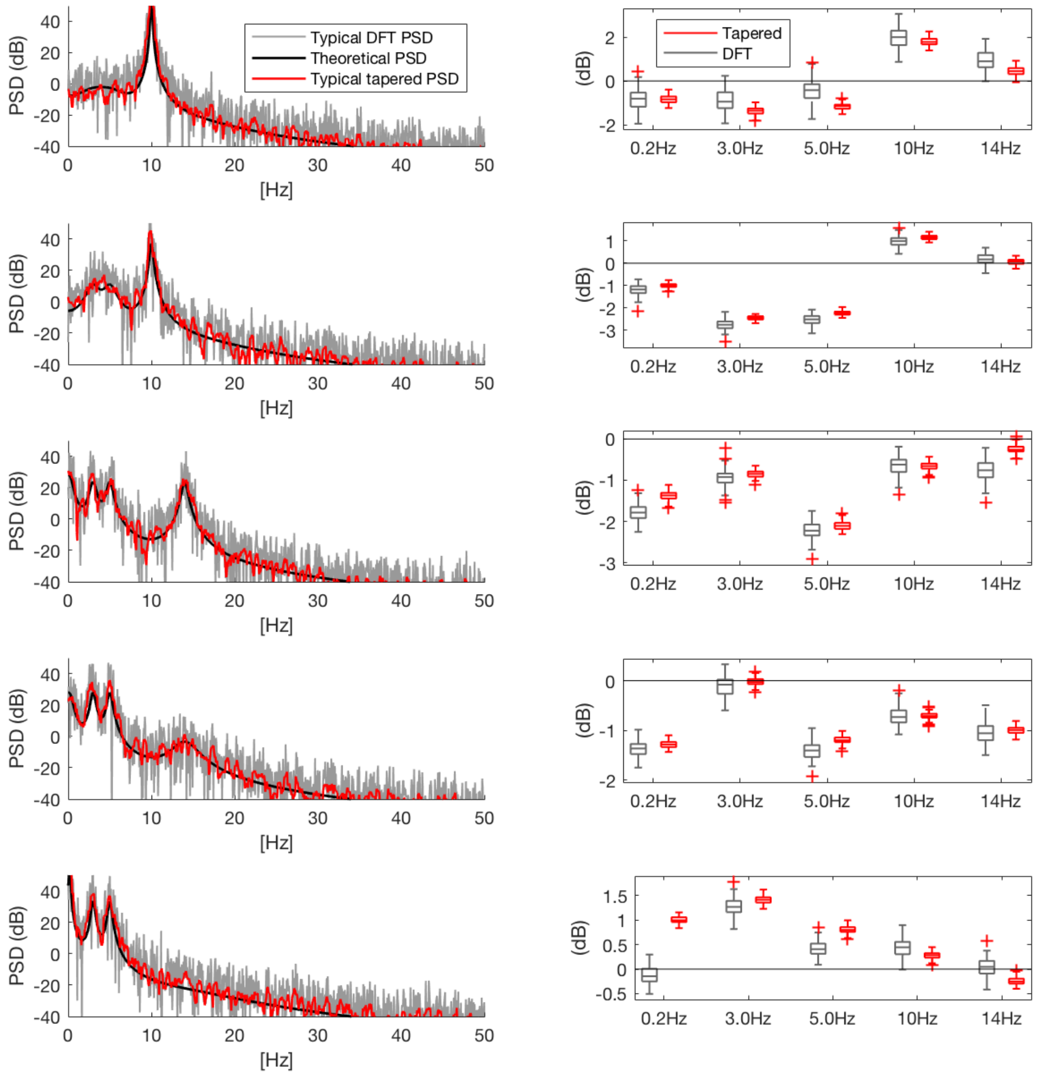


Figure S2: Left : power spectral densities. Theoretical PSD (black), periodogram (grey) and tapered estimates (red) are computed on the same 15s time window. Right : boxplots computed on the samples of the difference (in dB) using discrete Fourier transform (grey), or multitapered analysis (red).

# 3 Additional Details: Clustering

## 3.1 Cluster Characteristics (Figure S1)

Nine clusters were chosen based on the point at which the within-cluster point-to-center distance reached a local minimum. Figure S1 shows the spectral characteristics of the nine identified cluster

centers. For comparison, the spectral characteristics of each of the sleep expert scored stages is also shown, as an average of the distribution of power in all windows labeled as each of those states. Each cluster mimics the spectral signature of at least one of the sleep expert scored stages, which suggests that the spectral signatures represented by the clusters have physiological validity. However, the clusters capture a much wider range of distributions of power than the sleep expert scored stages, indicating that perhaps the clusters are sensitive to dynamics that are faster, more nuanced, or specific to certain subpopulations of subjects.

### 3.2 Cluster Dominance Across All Subjects (Table S1)

Table S1 contains details on how often each cluster was the most dominant during each scored sleep stage across all 14 nights of data. For each night, a cluster was considered 'dominant' if it was present for more than 50 percent of any sleep stage. Two clusters were considered jointly dominant (and both counted) if each was present for more than 40 percent of any sleep stage. Cluster 2 was the only cluster that was never dominant in any stage of sleep across all nights of data.

Table S1: Cluster Dominance by Sleep Stage Across All Nights

| | NREM3 | NREM2 | NREM1 | REM | Wake |
|---|---|---|---|---|---|
| Cluster 6 | **9** | **1** | 0 | 0 | 0 |
| Cluster 1 | **6** | **2** | 0 | 0 | 0 |
| Cluster 7 | 0 | **6** | **4** | 0 | 0 |
| Cluster 4 | 0 | **6** | **6** | **10** | 0 |
| Cluster 8 | 0 | 0 | **1** | **5** | 0 |
| Cluster 3 | 0 | 0 | 0 | 0 | **1** |
| Cluster 2 | 0 | 0 | 0 | 0 | 0 |
| Cluster 9 | 0 | 0 | 0 | 0 | **4** |
| Cluster 5 | 0 | 0 | 0 | 0 | **2** |

**Stage-Specific Cluster Transition Rate for Subjects 3 and 7 (Table S2)** Table S2 contains the computed number of cluster transitions per minute within each sleep expert scored stage for two subjects, 3 and 7.

Table S2: Cluster transitions per minute by sleep stage for Subjects 3 and 7

| | NREM3 | NREM2 | NREM1 | REM | Wake |
|---|---|---|---|---|---|
| Subject 3 | 0.99 | 0.45 | 0.16 | 0.04 | 0.26 |
| Subject 7 | 0.06 | 0.45 | 0.59 | 0.30 | 0.63 |

## References

[1] Robert H. Shumway and David S. Stoffer. *Time Series Analysis and Its Applications*. Springer Texts in Statistics. Springer International Publishing, Cham, 2017.
